# Supplementary material for: Online Estimation of Self-Body Deflection With Various Sensor Data Based on Directional Statistics
Source: arXiv:2306.03616 source file (2023-06-06)
Supplement: Supplementary file 1 [file A_appendix.tex]

\section*{APPENDIX}

\subsection{Changes in apparent rigidity} \label{appendix:apparent-rigidity}
% Appendixes should appear before the acknowledgment.

For simplicity, consider the deflection of a 1-link 1-joint robot arm.
This can be thought as a cantilever as shown in \figref{figure:appendix-link}. 
% Below, when varphi = 0 as shown in Fig. 12. 
Here we let $\varphi = 0$ as shown in \figref{figure:appendix-cantilever}.
Consider the max of deflection and assume that the angle of deflection is small enough.

Let the specific weight of the material be $\gamma$, Young's modulus be $E$, cross-sectional area be $A$, link length (beam length) be $L$, and moment of inertia of area be $I$. The max of deflection of the beam due to its own weight, which denotes $\delta_{\max}$, is computed as follows \cite{Gross2017:material}.
\begin{align}
    \delta_{\max }=\frac{\gamma A L^{4}}{8 E I}.
    \label{equ:appendix:deltamax}
\end{align}
When the scale is multiplied by $k$ keeping the material and structure, that is, without changing $E$ and $\gamma$,
\begin{align}
    L \mapsto k L, \quad A \mapsto k^{2} A, \quad I \mapsto k^{4} I.
\end{align}
Therefore, after scaling, $\delta_{\max}$ becomes
\begin{align}
    \delta_{\max } \mapsto \frac{\gamma \cdot\left(k^{2} A\right) \cdot(k L)^{4}}{8 E \cdot\left(k^{4} I\right)}=k^{2} \delta_{\max }.
\end{align}
The ratio of the maximum amount of deflection to the link length $\delta_{\max}^* := \delta_{\max} / L$ becomes
\begin{align}
    \delta_{\mathrm{max}}^{*}=\frac{\delta_{\mathrm{max}}}{L} \mapsto \frac{k^{2} \delta_{\mathrm{max}}}{k L}=k \delta_{\mathrm{max}}^{*}.
    \label{equ:appendix:deltamaxstar}
\end{align}
% \TODO{fix google translate}
The rightmost value of \equref{equ:appendix:deltamaxstar} coincides with the value obtained by multiplying Young's modulus $E$ by $k^{-1}$ in \equref{equ:appendix:deltamax} while keeping the scale invariant.
This implies that the ``apparent Young's modulus'' decreases as the size of a robot increases.
% The above discussion was about 
We discussed above 1-link and 1-joint robot arm, but in an actual robot, multiple links are connected and the elasticity of the joint itself is also taken into consideration. Therefore it is thought that even greater deflection will occur.

% This is equal to the value obtained by multiplying the Yung's modulus E by k-1 in Eq. (7) with the scale invariance. This suggests that the apparent Young's modulus decreases with increasing size. ..
% The above discussion was about 1 link and 1 joint, but in an actual robot, multiple links are connected and the elasticity of the joint itself is also taken into consideration, so it is thought that even greater deflection will occur.

% This is equal to the value obtained by multiplying the Yung's modulus E by k-1 in Eq. (7) with the scale invariance. This suggests that the apparent Young's modulus decreases with increasing size. ..
% The above discussion was about 1 link and 1 joint, but in an actual robot, multiple links are connected and the elasticity of the joint itself is also taken into consideration, so it is thought that even greater deflection will occur.
\begin{figure}[t]
    \centering
    \includegraphics[width=0.75\linewidth]{figs/cantilever-and-link.eps}
    % \vspace{-3mm}
    \caption{The joint-and-link model and its equivalent cantilever model}
    \label{figure:appendix-link}
\end{figure}
\begin{figure}[t]
    \centering
    \includegraphics[width=0.95\linewidth]{figs/cantilever-weight.pdf}
    % \vspace{-3mm}
    \caption{The cantilever subjected to the uniformly distributed load $\gamma A$ which is caused by its weight}
    \label{figure:appendix-cantilever}
\end{figure}
